# Supplementary material for: Functionality understanding and segmentation in 3D scenes
Source: arXiv:2411.16310 source file (2025-05-28)
Supplement: Supplementary file 2 [file mypackages.tex]

\usepackage[dvipsnames]{xcolor}
\usepackage{amsmath,amssymb,amsfonts}
\usepackage{multirow,multicol}
\usepackage{natbib}
\usepackage{algorithmic}
\usepackage{graphicx}
\usepackage{textcomp}
\usepackage{xspace}
\usepackage{url}
\usepackage{dsfont}
\usepackage{booktabs}
\usepackage{balance}
\usepackage{soul}
\usepackage{todonotes}
\usepackage{pifont}
\usepackage{colortbl}
\usepackage{overpic}
\usepackage{enumitem}
\usepackage{nccmath}
\usepackage{courier}
\usepackage{array}% http://ctan.org/pkg/array
\usepackage{tabularray}
\usepackage{pifont}% http://ctan.org/pkg/pifont
\usepackage[accsupp]{axessibility} % Improves PDF readability for those with visual impairments.
\usepackage{pgfplots}
\pgfplotsset{compat=1.18}
\usepackage{comment}
\usepackage{microtype}
\usepackage{transparent}
\usepackage[export]{adjustbox}
